# Supplementary material for: Topological tuning in three-dimensional Dirac semimetals
Source: arXiv:1408.3509 source file (2014-12-17)
Supplement: Supplementary file 1 [file supplement_na3bi.pdf]

# Supplemental Material: Topological tuning in three-dimensional Dirac semimetals

Awadhesh Narayan
*School of Physics and CRANN, Trinity College, Dublin 2, Ireland*

Domenico Di Sante
*Consiglio Nazionale delle Ricerche (CNR-SPIN), Via Vetoio, L'Aquila, Italy and*
*Department of Physical and Chemical Sciences, University of L'Aquila, Via Vetoio 10, I-67010 L'Aquila, Italy*

Silvia Picozzi
*Consiglio Nazionale delle Ricerche (CNR-SPIN), Via Vetoio, L'Aquila, Italy*

Stefano Sanvito
*School of Physics, CRANN and AMBER, Trinity College, Dublin 2, Ireland*
(Dated: October 27, 2014)

In this supplement we elaborate on (i) an alloying-induced topological phase transition in $Cd_3[P_{1-x}As_x]_2$, and (ii) a general low-energy Dirac-like Hamiltonian for three-dimensional Dirac semimetals to study this transition.

## ALLOYING INDUCED TRANSITION IN $\mathbf{Cd_3[P_{1-x}As_x]_2}$

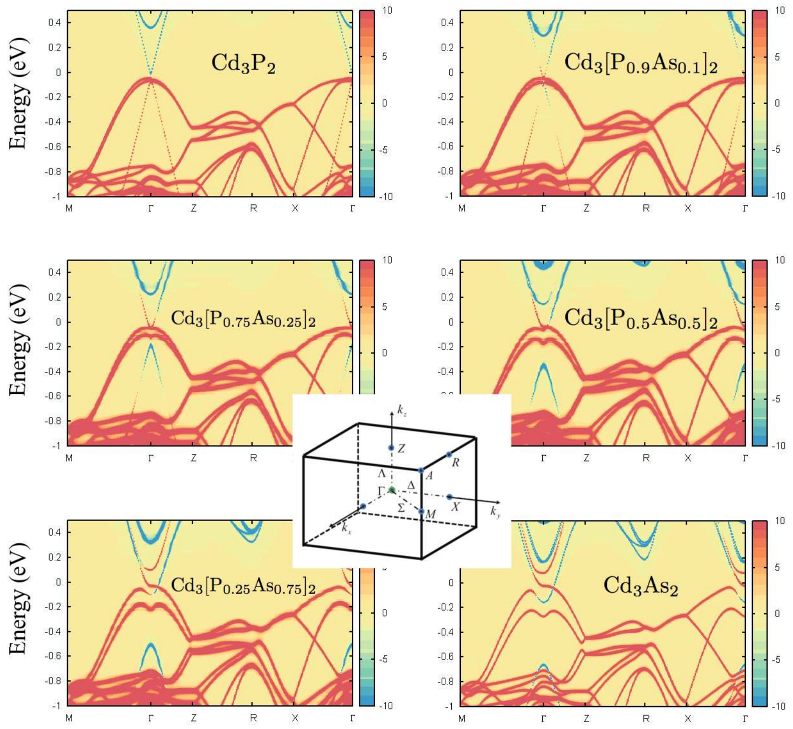


FIG. 1: Spectral functions for the alloy $Cd_3[P_{1-x}As_x]_2$ with increasing As concentration ($x = 0.0, 0.10, 0.25, 0.50, 0.75, 1.0$ from top to bottom and from left to right). The color scale shows the orbital contribution, with red (positive values) denoting P/As $p$ orbitals and blue (negative values) representing Cd $s$ orbitals (in units of states/eV). The central inset shows the tetragonal Brillouin zone of the $P4_2$/nmc space group.

In addition to $Na_3Bi$, also $Cd_3As_2$ has been observed to show a three dimensional Dirac semimetal state. We predict that, analogously to $Na_3Bi_{1-x}Sb_x$ alloys, a similar topological phase transition can be observed in $Cd_3[P_{1-x}As_x]_2$. In order to study the alloying-induced topological transition in the $Cd_3[P_{1-x}As_x]_2$ alloys, we consider both pristine

compounds, i.e. $Cd_3P_2$ and $Cd_3As_2$, in their P$4_2$/nmc space group structure [2, 3]. We note here that $Cd_3As_2$ has been recently predicted to crystallize at ambient conditions into the I$4_1$/acd space group, a $\sqrt{2}\times\sqrt{2}\times 2$ supercell of the P$4_2$/nmc structure [4]. However, low-energy features are robust against the choice of the space group, as can be inferred by comparing bandstructures reported in Refs. [2] and [4], so that we perform our simulations for the smaller P$4_2$/nmc cell.

In Fig. 1 we report our CPA calculations for $Cd_3[P_{1-x}As_x]_2$ alloys, highlighting that $Cd_3P_2$ shows a trivial gap of $\sim 50$ meV, while in $Cd_3As_2$ a topological bulk band crossing occurs along the $\Gamma - Z$ line at the Fermi level. Our calculations reveal that a small concentration of As, namely $x = 0.10$, is sufficient to achieve the topological bulk gap closure. Furthermore, we note also that the low-energy features around the 3D Dirac cone are protected against the broadening action of disorder, preserving their quasiparticle nature [5], and for this reason they should be clearly detectable in angle-resolved photoemission experiments.

These results for $Cd_3[P_{1-x}As_x]_2$ alloys are analogous to those reported for $Na_3Bi_{1-x}Sb_x$ alloys, as detailed in the main manuscript. However, $Na_3Bi$ and $Na_3Sb$ are unstable in air and special care is needed to prepare the samples. In contrast, $Cd_3As_2$ and $Cd_3P_2$ are stable in atmosphere conditions. Moreover, $Cd_3As_2$ is known to have very high mobility, which we also expect the alloys to inherit.

## LOW-ENERGY HAMILTONIAN AND TOPOLOGICAL PHASE TRANSITION

A minimal $4 \times 4$ low-energy Hamiltonian for the Dirac semimetal around the Brillouin zone center ($\Gamma$) can be written down as [1, 2]

$$\mathcal{H}(\mathbf{k}) = \epsilon_0(\mathbf{k})\mathbb{I} + \begin{pmatrix} M(\mathbf{k}) & Ak_+ & 0 & B^*(\mathbf{k}) \\ Ak_- & -M(\mathbf{k}) & B^*(\mathbf{k}) & 0 \\ 0 & B(\mathbf{k}) & M(\mathbf{k}) & -Ak_- \\ B(\mathbf{k}) & 0 & -Ak_+ & -M(\mathbf{k}) \end{pmatrix}, \tag{1}$$

where $\epsilon_0(\mathbf{k}) = C_0 + C_1 k_z^2 + C_2(k_x^2 + k_y^2)$, $\mathbb{I}$ is a $4\times 4$ identity matrix, $k_\pm = k_x \pm i k_y$, $M(\mathbf{k}) = m_0 - m_1 k_z^2 - m_2(k_x^2 + k_y^2)$, and $B(\mathbf{k}) = B_3 k_z k_+^2$. Here the basis is $[|S^+, 1/2\rangle, |P^-, 3/2\rangle, |S^-, 1/2\rangle, |P^-, 3/2\rangle]$, with $S$ and $P$ denoting the hybrid states from the Na and the Bi atoms, the superscript $\pm$ labels the parity and the second number in the ket vector denotes the total angular momentum. We use the following parameters for $Na_3Bi$, obtained by fitting to first-principles results [1]: $C_0 = -63.82$ meV, $C_1 = 8.7536$ eVÅ$^2$, $C_2 = -8.4008$ eVÅ$^2$, $m_1 = -10.6424$ eVÅ$^2$, $m_2 = -10.3610$ eVÅ$^2$, and $A = 2.4598$ eVÅ. We then tune the value of the mass parameter, $m_0$, to obtain the phase transition as shown in Fig. 2. The two Dirac nodes move towards the $\Gamma$ point as the mass is increased ($m_0$ is tuned towards zero from negative values), they meet at the critical point $m_0 = 0$ and then a trivial gap opens up in the spectrum for $m_0 > 0$. This well models our density functional theory and coherent potential approximation results for $Na_3Bi_{1-x}Sb_x$ alloy presented in the main paper.

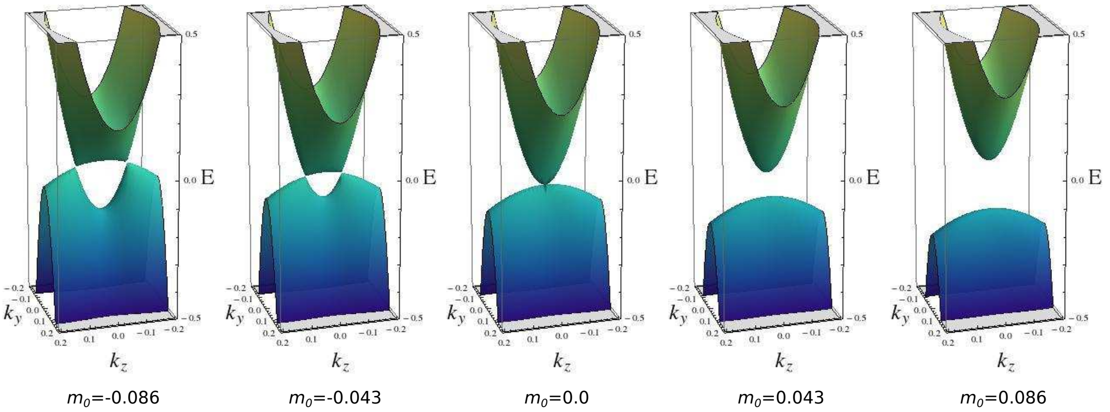


FIG. 2: Band structure for the effective low-energy Dirac model as a function of the mass term, showing the topological transition from Dirac semimetal to a trivial insulator. Note the shifting of the Dirac crossing towards $\Gamma$ as the mass is increased to zero.

[1] Z. Wang, Y. Sun, X.-Q. Chen, C. Franchini, G. Xu, H. Weng, X. Dai, and Z. Fang, Phys. Rev. B **85**, 195320 (2012).
[2] Z. Wang, H. Weng, Q. Wu, X. Dai, and Z. Fang, Phys. Rev. B **88**, 125427 (2013).
[3] U. Paliwal and K.B. Joshi, Physica B **406**, 3060 (2011).
[4] M.N. Ali, Q. Gibson, S. Jeon, B.B. Zhou, A. Yazdani and R.J. Cava, Inorg. Chem. **53**, 4062 (2014).
[5] D. Di Sante, P. Barone, E. Plekhanov, S. Ciuchi, and S. Picozzi, arXiv:1407.2064.
